# Supplementary material for: Historian: Reducing Manual Validation in APR Benchmarking via Evidence-Based Assessment
Source: arXiv:2603.00649 source file (2026-02-28)
Supplement: Supplementary file 1 [file appendix.tex]

% Against Pre
\begin{figure*}[ht]
    \centering
    \includegraphics[width=0.9\textwidth]{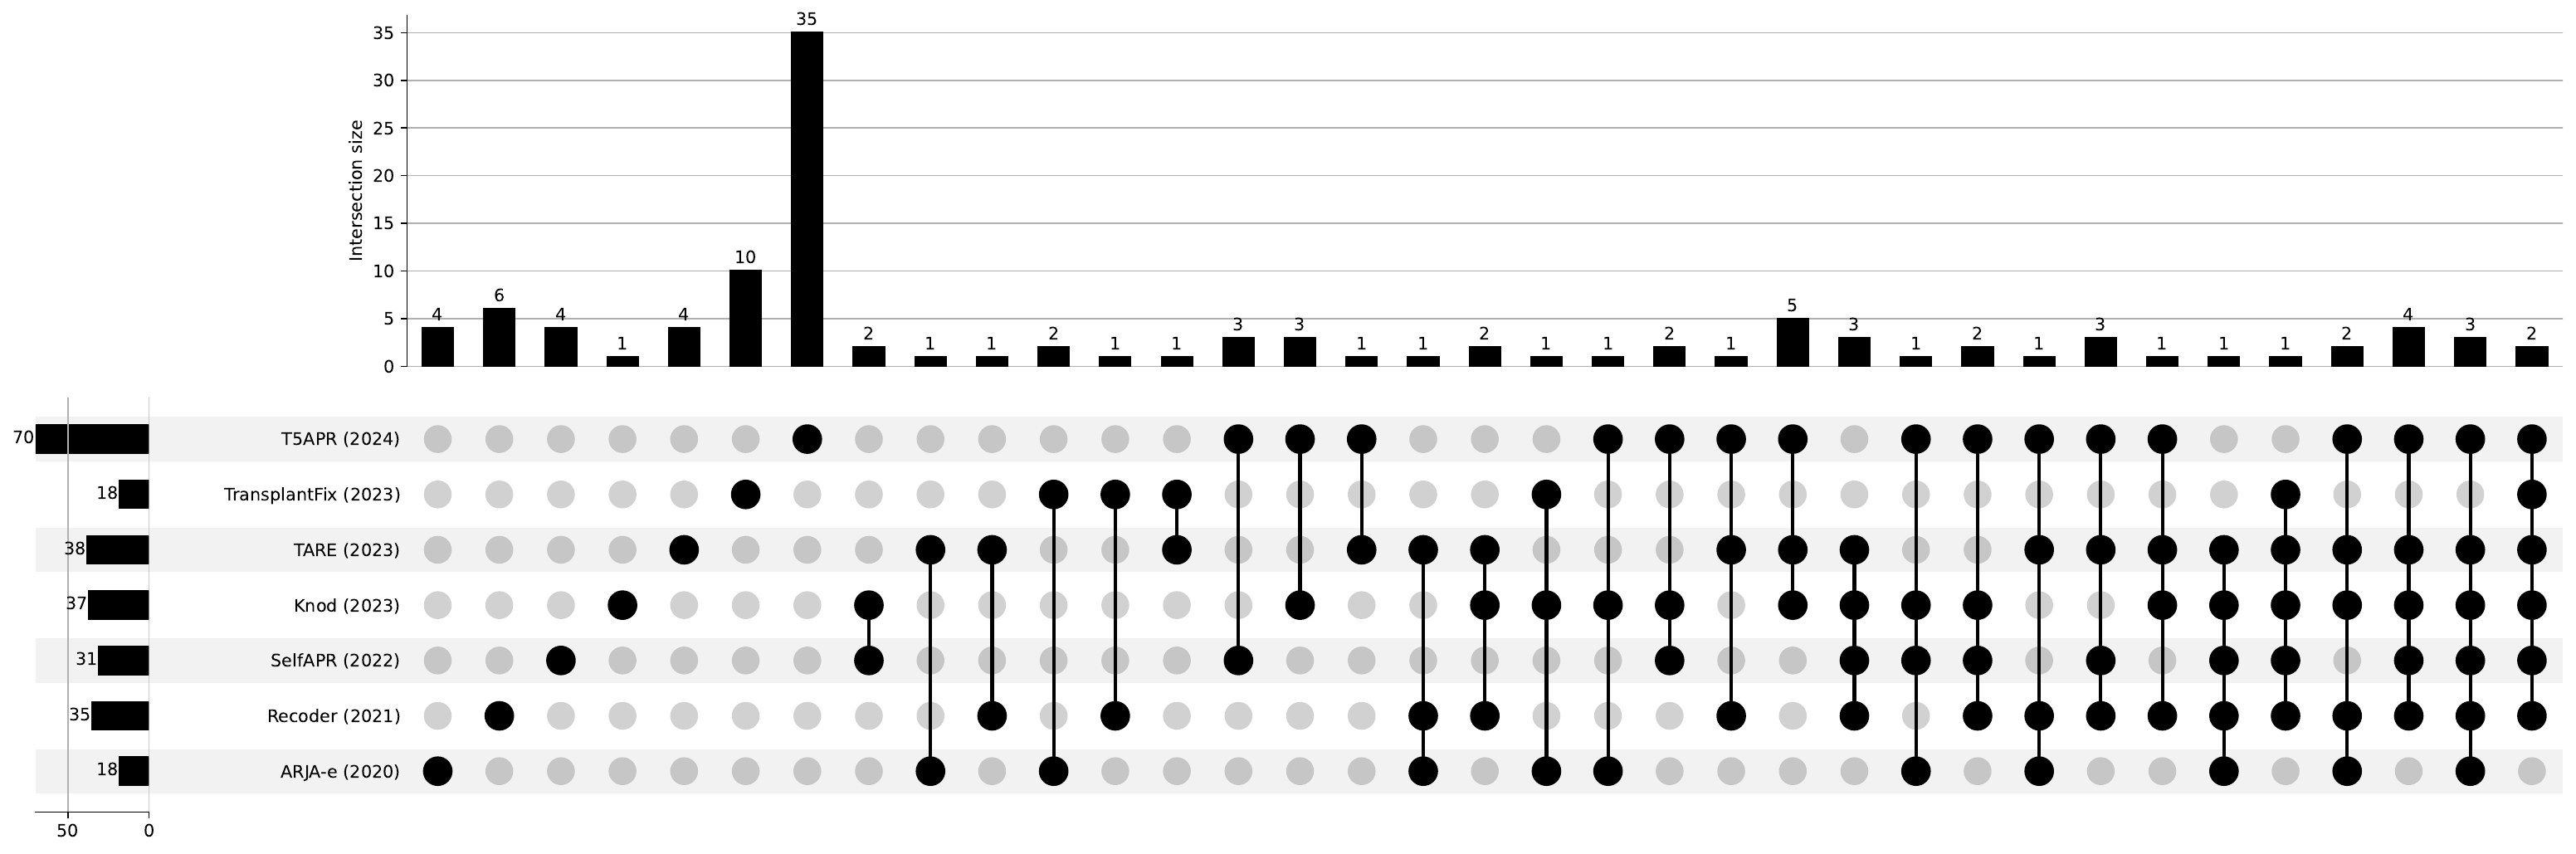}
    \vspace{-0.5em}
    \caption{Upset Diagram of Correct Baseline Patches}
    \label{fig:upset_baseline_vs_correct}
\end{figure*}

\begin{figure*}[ht]
    \centering
    \includegraphics[width=0.9\textwidth]{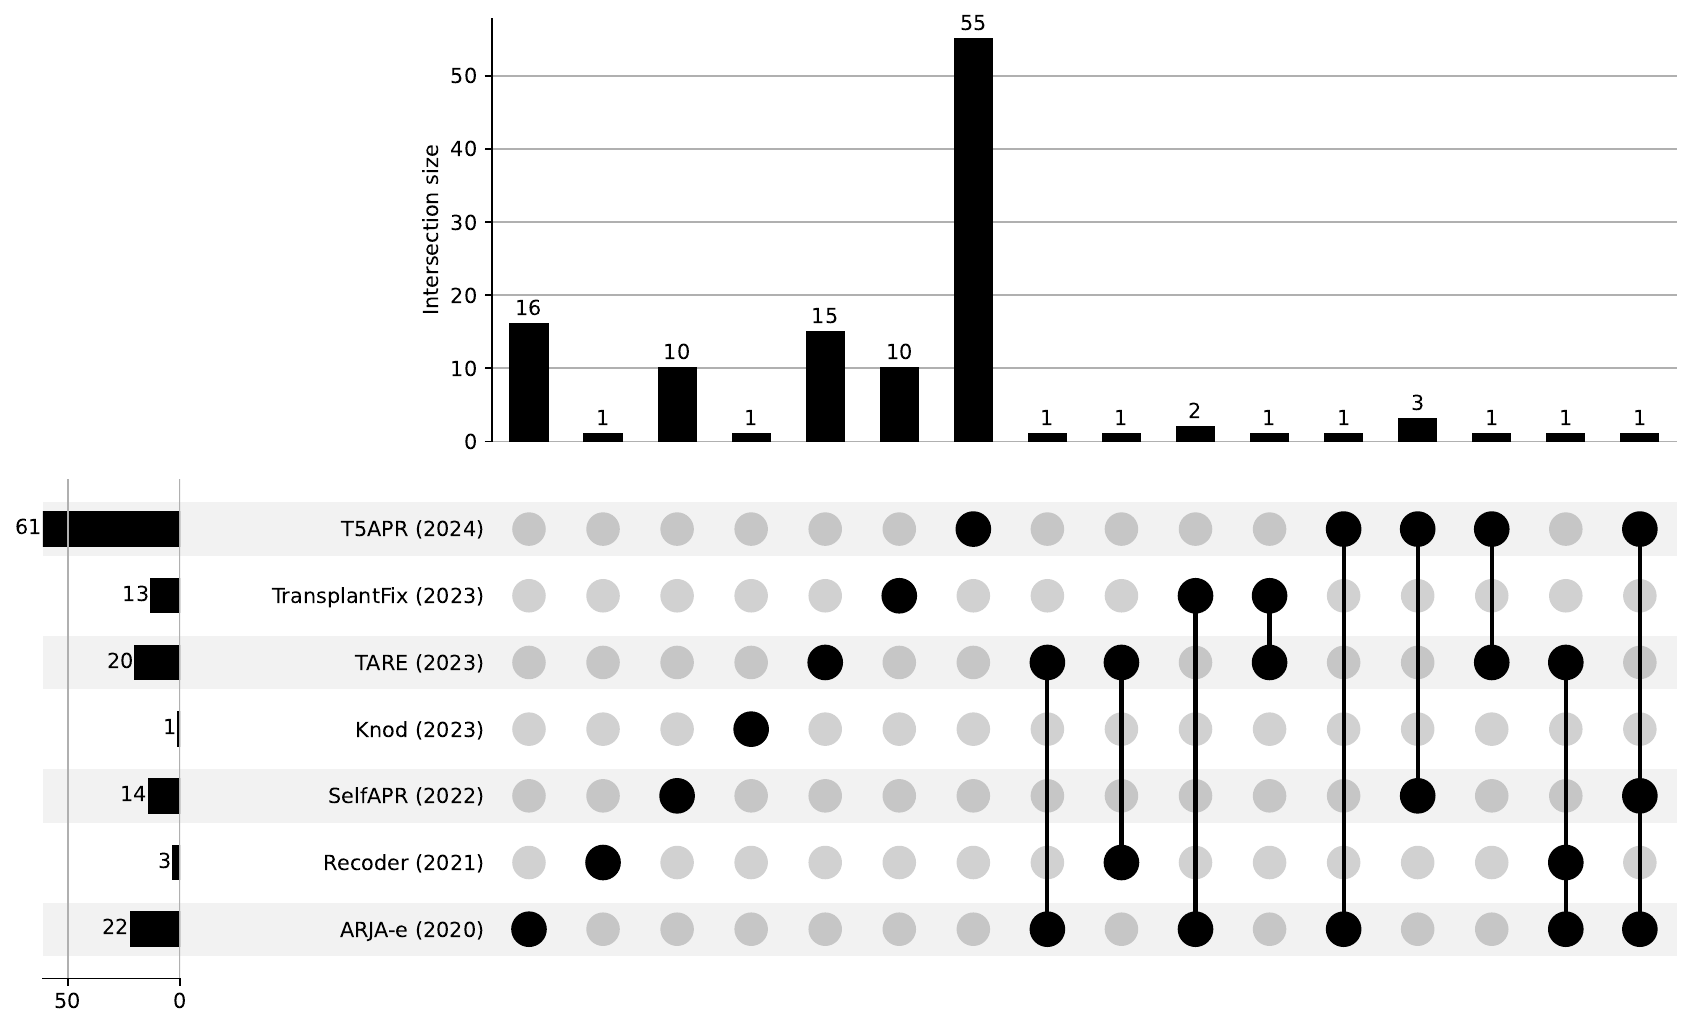}
    \vspace{-0.5em}
    \caption{Upset Diagram of Overfitting Baseline Patches}
    \label{fig:upset_baseline_vs_overfitting}
\end{figure*}

% % include all
% \begin{figure*}[ht]
%     \centering
%     \includegraphics[width=0.9\textwidth]{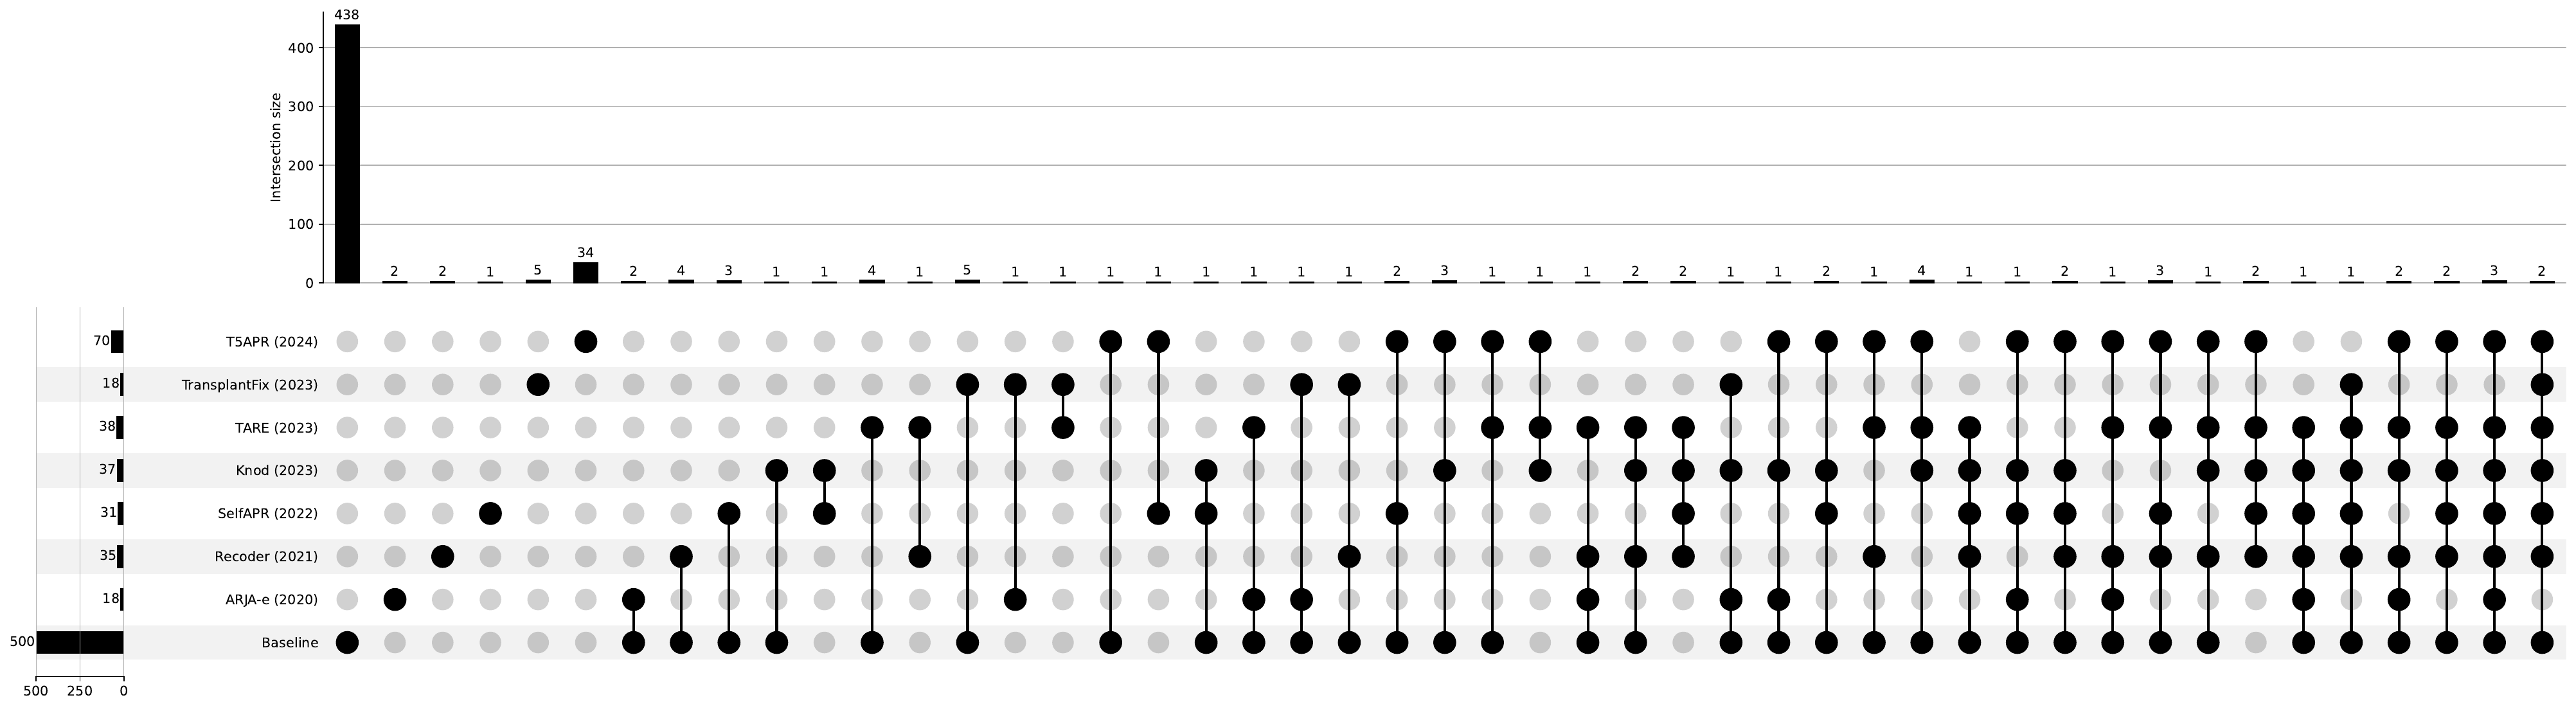}
%     \vspace{-0.5em}
%     \caption{Upset Diagram of Correct Baseline Patches and Tool Patches}
%     \label{fig:upset_all_correct}
% \end{figure*}

% \begin{figure*}[ht]
%     \centering
%     \includegraphics[width=0.9\textwidth]{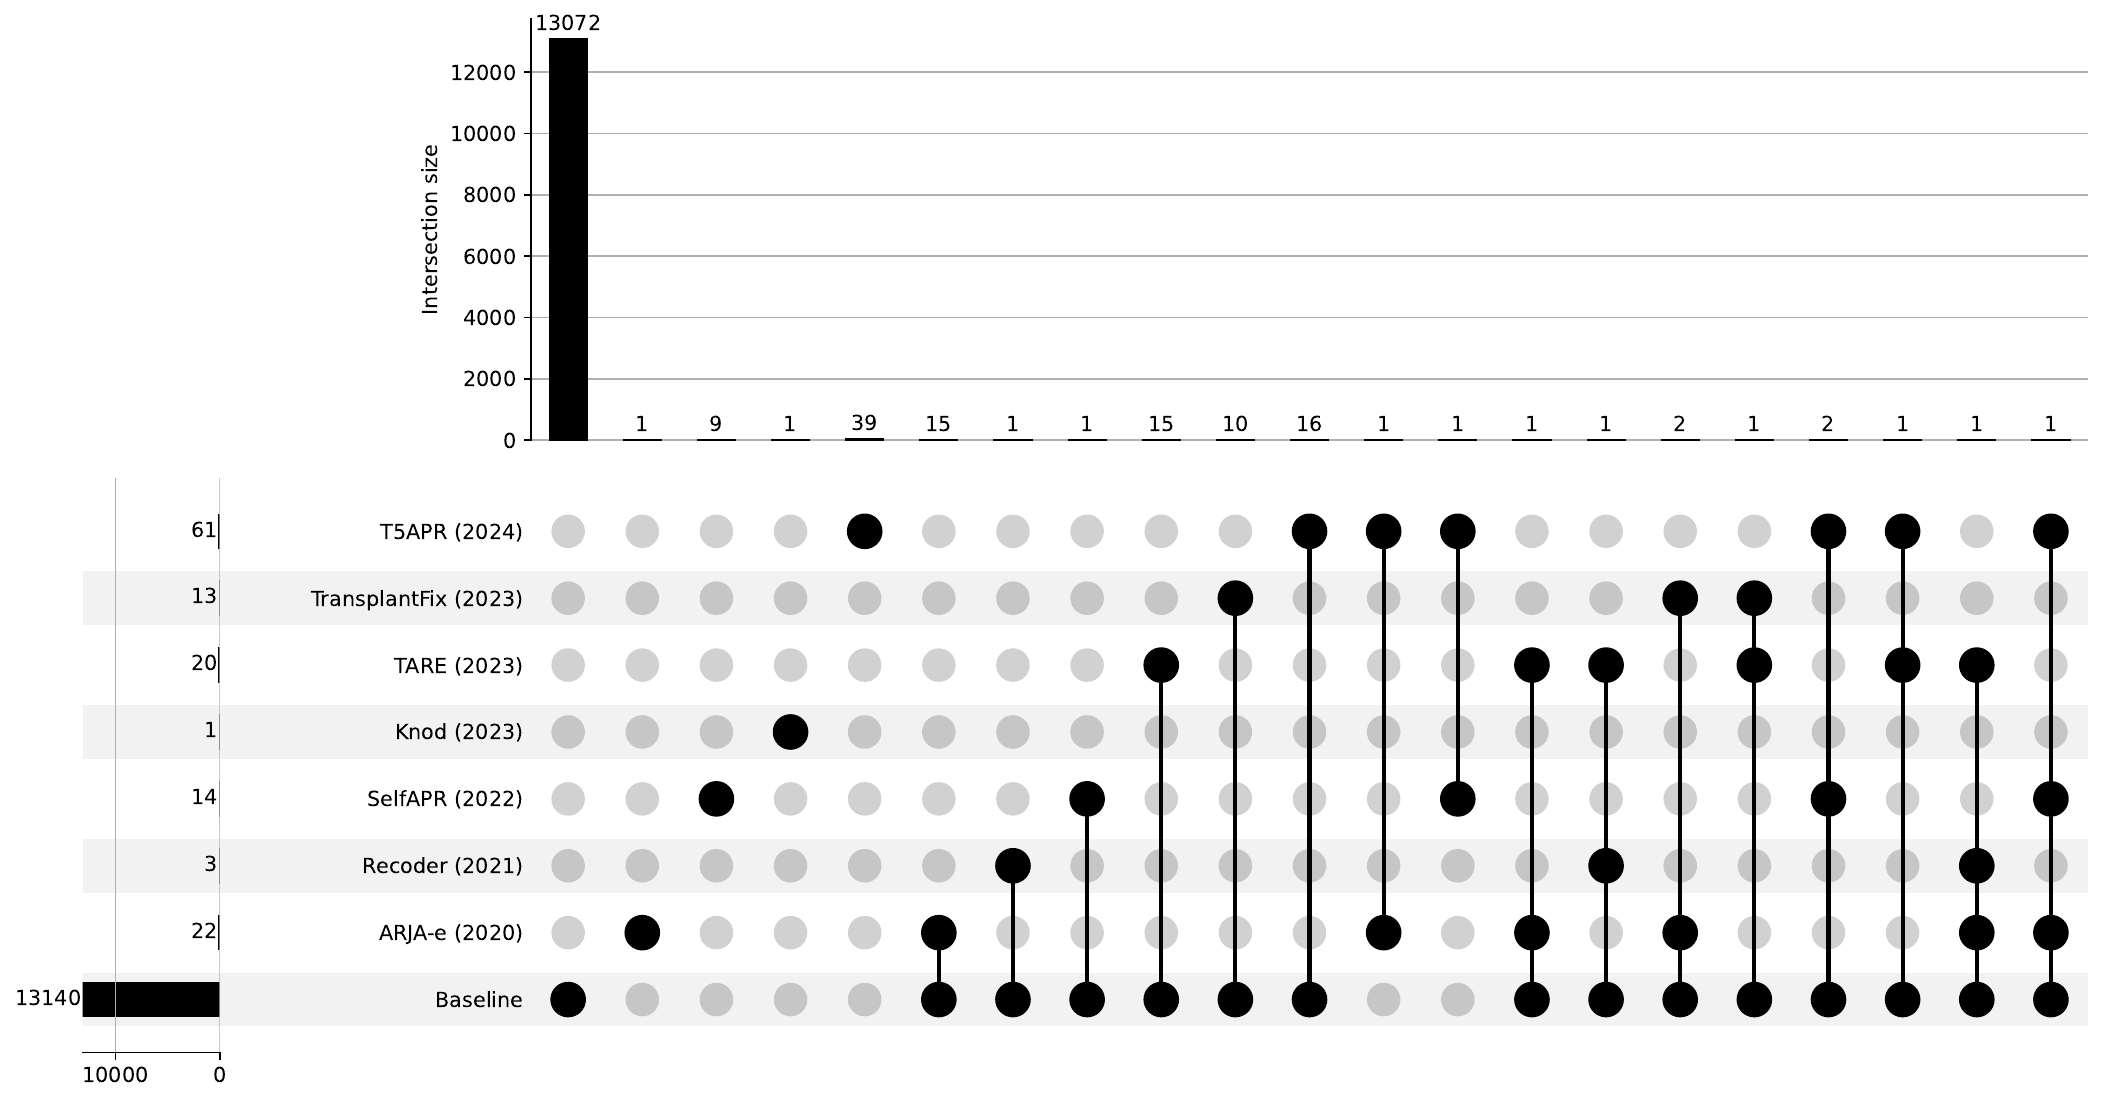}
%     \vspace{-0.5em}
%     \caption{Upset Diagram of Overfitting Baseline Patches and Tool Patches}
%     \label{fig:upset_all_overfitting}
% \end{figure*}

% include T5APR
\begin{figure*}[ht]
    \centering
    \includegraphics[width=0.9\textwidth]{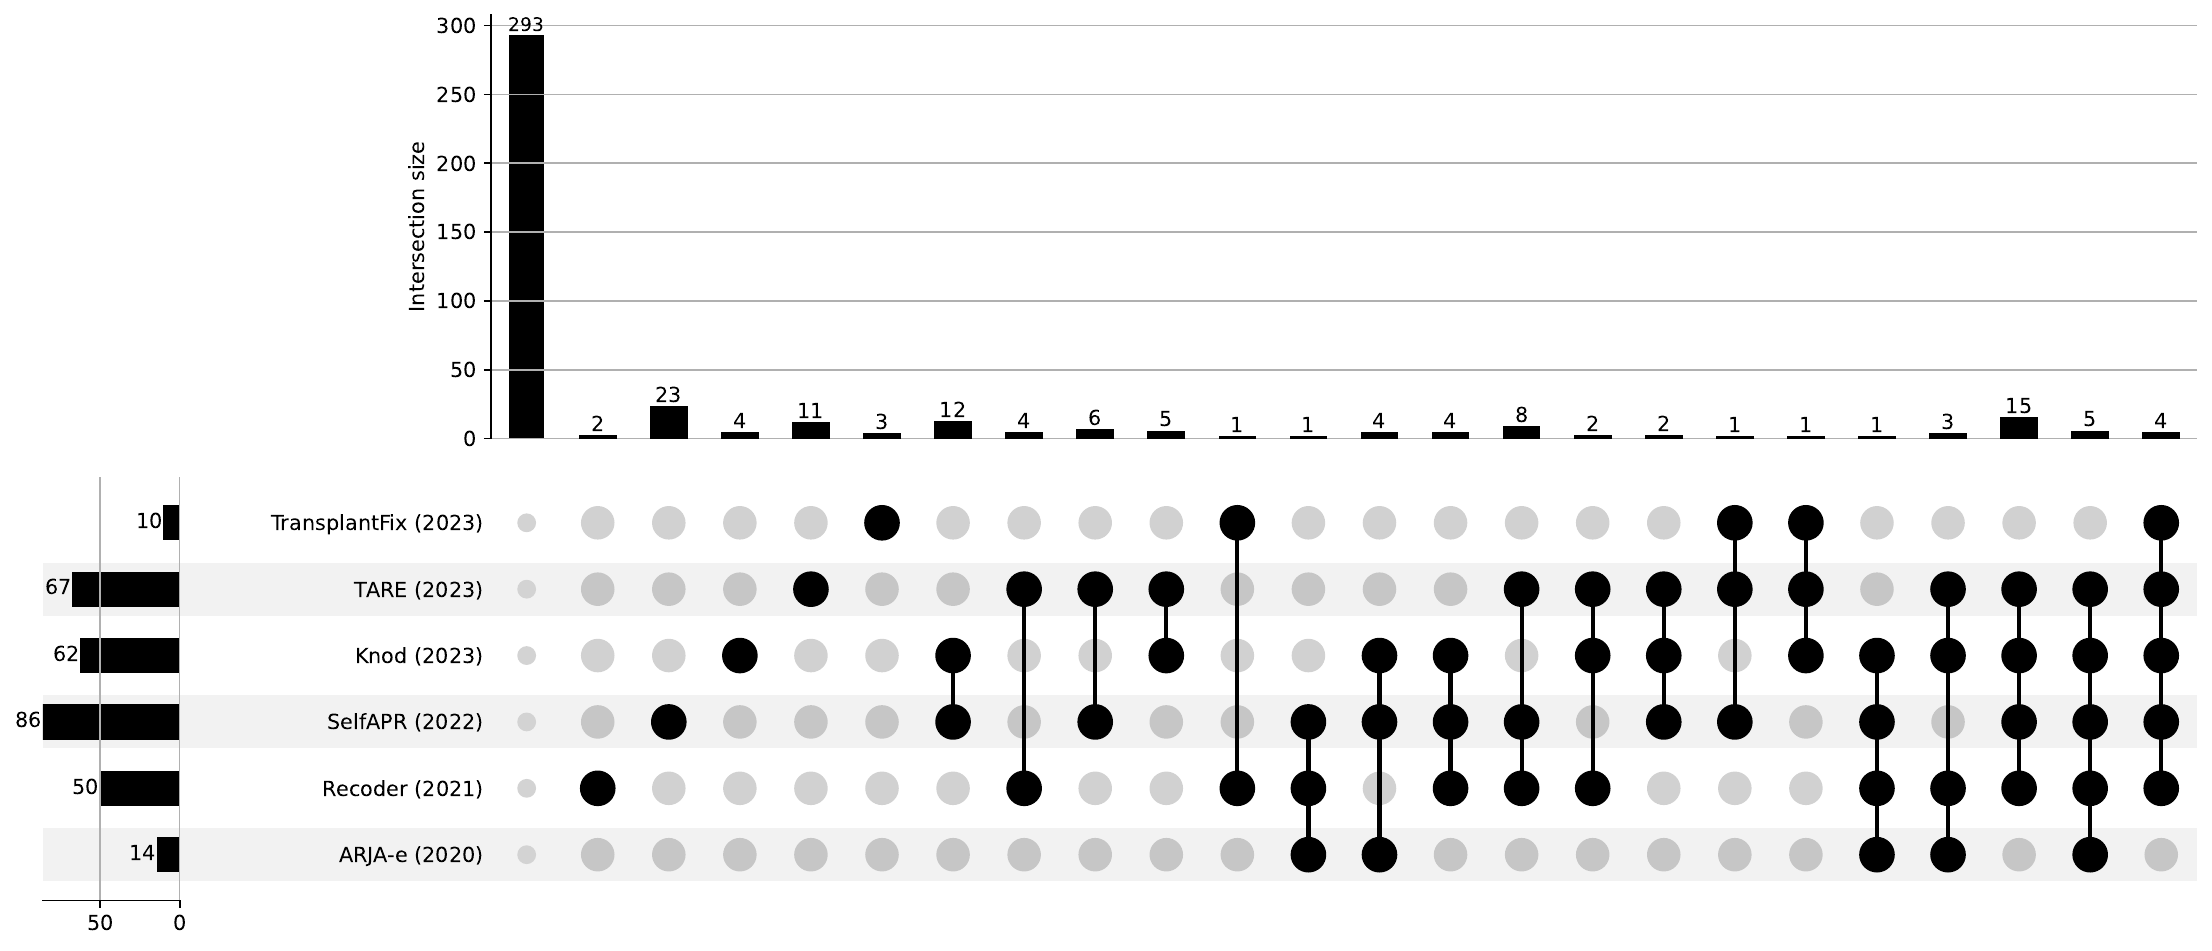}
    \vspace{-0.5em}
    \caption{Upset Diagram of 122 Matching T5APR Correct Patches Across Tools}
    \label{fig:upset_t5apr_included_correct}
\end{figure*}

\begin{figure*}[ht]
    \centering
    \includegraphics[width=0.9\textwidth]{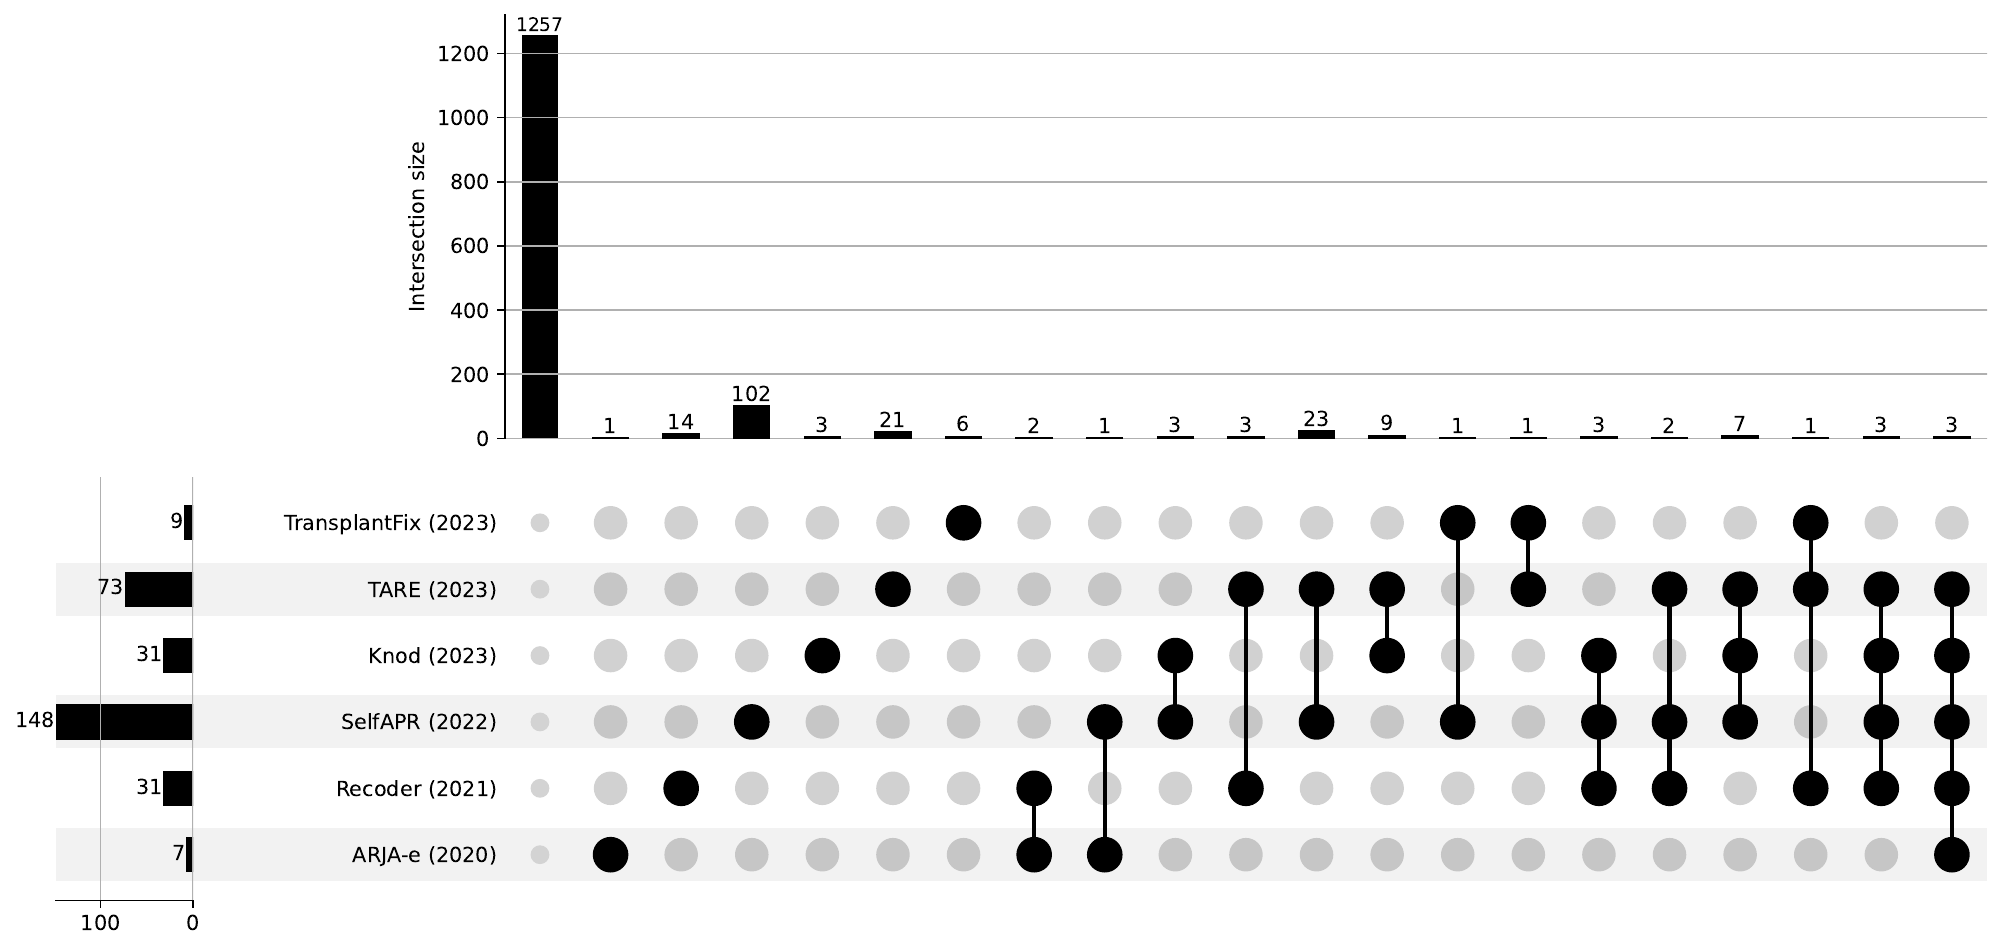}
    \vspace{-0.5em}
    \caption{Upset Diagram of 209 Matching T5APR Overfitting Patches Across Tools}
    \label{fig:upset_t5apr_included_overfitting}
\end{figure*}

\section{Appendix}
\label{sec:appendix}

\begin{longtable}{l|c|l|l|c}
\caption{Oracle Experiment Results: Expert-Labeled Clone Types to Patch Correctness Verdicts for TBar Patches}
\label{tab:oracle-results} \\
\hline
\textbf{TBar Patch} & \textbf{Pairs} & \textbf{Clone Labels} & \textbf{Verdicts} & \textbf{Pred.} \\
\hline
\endfirsthead

\multicolumn{5}{c}%
{{\tablename\ \thetable{} -- continued from previous page}} \\
\hline
\textbf{TBar Patch} & \textbf{Pairs} & \textbf{Clone Labels} & \textbf{Verdicts} & \textbf{Pred.} \\
\hline
\endhead

\hline
\multicolumn{5}{r}{{Continued on next page}} \\
\endfoot 

\hline
\multicolumn{5}{l}{\footnotesize 
\textbf{Clone Labels:} T1-T4: Type-1 to Type-4, NC: Not-Clone. \quad
\textbf{Verdicts:} C: Correct, O: Overfitting, U: Unknown.} \\
\multicolumn{5}{l}{\footnotesize 
\textcolor{green!60!black}{Green}: Correct prediction, \textcolor{orange}{Orange}: Overfitting prediction, \textcolor{gray}{Gray}: Unknown.} \\
\endlastfoot

Chart-1-TBar-Patch\_2781\_1214 & 68 & T1:15, T3:4, NC:49 & C:15, U:53 & \textcolor{green!60!black}{C} \\
Chart-11-TBar-Patch\_102\_60 & 12 & T1:7, T3:5 & C:7, U:5 & \textcolor{green!60!black}{C} \\
Chart-12-TBar-Patch\_39\_22 & 23 & T3:1, T4:3, NC:19 & O:6, U:17 & \textcolor{orange}{O} \\
Chart-13-TBar-Patch\_29\_18 & 55 & T3:3, NC:52 & O:1, U:54 & \textcolor{orange}{O} \\
Chart-14-TBar-Patch\_2034\_473 & 55 & T2:1, T3:11, NC:43 & O:5, U:50 & \textcolor{orange}{O} \\
Chart-14-TBar-Patch\_2631\_615 & 55 & T1:1, T3:14, NC:40 & O:5, U:50 & \textcolor{orange}{O} \\
Chart-14-TBar-Patch\_2669\_616 & 55 & T2:1, T3:13, NC:41 & O:3, U:52 & \textcolor{orange}{O} \\
Chart-14-TBar-Patch\_974\_207 & 55 & T3:16, T4:1, NC:38 & O:4, U:51 & \textcolor{orange}{O} \\
Chart-15-TBar-Patch\_220\_119 & 44 & T1:2, T3:31, NC:11 & O:2, U:42 & \textcolor{orange}{O} \\
Chart-19-TBar-Patch\_143\_118 & 9 & T3:7, NC:2 & U:9 & \textcolor{gray}{U} \\
Chart-19-TBar-Patch\_68\_59 & 9 & T1:4, T4:3, NC:2 & C:7, U:2 & \textcolor{green!60!black}{C} \\
Chart-24-TBar-Patch\_42\_20 & 12 & T1:6, T4:5, NC:1 & C:11, U:1 & \textcolor{green!60!black}{C} \\
Chart-25-TBar-Patch\_12\_9 & 99 & T1:2, T3:31, NC:66 & O:2, U:97 & \textcolor{orange}{O} \\
Chart-26-TBar-Patch\_5751\_2399 & 16 & T3:12, NC:4 & O:2, U:14 & \textcolor{orange}{O} \\
Chart-3-TBar-Patch\_440\_242 & 20 & T1:1, T3:2, T4:1, NC:16 & O:6, U:14 & \textcolor{orange}{O} \\
Chart-4-TBar-Patch\_2689\_1263 & 4 & T1:3, NC:1 & C:3, U:1 & \textcolor{green!60!black}{C} \\
Chart-5-TBar-Patch\_52\_1 & 23 & T3:2, NC:21 & O:4, U:19 & \textcolor{orange}{O} \\
Chart-7-TBar-Patch\_2\_2 & 20 & T1:4, T2:1, T4:4, NC:11 & O:11, U:9 & \textcolor{orange}{O} \\
Chart-9-TBar-Patch\_497\_311 & 10 & T2:3, T3:3, NC:4 & C:3, U:7 & \textcolor{green!60!black}{C} \\
Closure-107-TBar-Patch\_356\_164 & 2 & NC:2 & O:1, U:1 & \textcolor{orange}{O} \\
Closure-109-TBar-Patch\_270\_73 & 6 & T1:2, T3:1, NC:3 & O:2, U:4 & \textcolor{orange}{O} \\
Closure-115-TBar-Patch\_704\_253 & 37 & T3:36, NC:1 & U:37 & \textcolor{gray}{U} \\
Closure-12-TBar-Patch\_160\_37 & 7 & T1:2, NC:5 & O:3, U:4 & \textcolor{orange}{O} \\
Closure-126-TBar-Patch\_6\_3 & 44 & T3:12, T4:1, NC:31 & O:12, U:32 & \textcolor{orange}{O} \\
Closure-133-TBar-Patch\_433\_171 & 5 & NC:5 & O:1, U:4 & \textcolor{orange}{O} \\
Closure-21-TBar-Patch\_260\_40 & 53 & T3:51, T4:2 & O:2, U:51 & \textcolor{orange}{O} \\
Closure-22-TBar-Patch\_5\_5 & 71 & T1:2, NC:69 & O:3, U:68 & \textcolor{orange}{O} \\
Closure-62-TBar-Patch\_43\_31 & 14 & T1:5, T3:9 & C:5, U:9 & \textcolor{green!60!black}{C} \\
Closure-66-TBar-Patch\_9\_6 & 4 & T1:2, NC:2 & O:3, U:1 & \textcolor{orange}{O} \\
Closure-73-TBar-Patch\_146\_58 & 10 & T1:8, T2:1, T3:1 & C:9, U:1 & \textcolor{green!60!black}{C} \\
Lang-10-TBar-Patch\_2435\_1012 & 8 & T3:3, T4:2, NC:3 & C:2, U:6 & \textcolor{green!60!black}{C} \\
Lang-13-TBar-Patch\_18\_6 & 4 & T1:2, NC:2 & O:2, U:2 & \textcolor{orange}{O} \\
Lang-18-TBar-Patch\_5849\_3524 & 3 & T1:2, NC:1 & O:3 & \textcolor{orange}{O} \\
Lang-20-TBar-Patch\_1220\_617 & 6 & T3:6 & U:6 & \textcolor{gray}{U} \\
Lang-20-TBar-Patch\_336\_182 & 6 & T3:6 & U:6 & \textcolor{gray}{U} \\
Lang-22-TBar-Patch\_1806\_847 & 24 & T3:24 & U:24 & \textcolor{gray}{U} \\
Lang-24-TBar-Patch\_2414\_1931 & 8 & T1:2, NC:6 & O:8 & \textcolor{orange}{O} \\
Lang-27-TBar-Patch\_1259\_919 & 18 & T1:2, NC:16 & O:3, U:15 & \textcolor{orange}{O} \\
Lang-33-TBar-Patch\_47\_28 & 8 & T3:8 & U:8 & \textcolor{gray}{U} \\
Lang-39-TBar-Patch\_1350\_1039 & 33 & T3:32, NC:1 & U:33 & \textcolor{gray}{U} \\
Lang-41-TBar-Patch\_289\_206 & 4 & T1:2, T3:2 & O:2, U:2 & \textcolor{orange}{O} \\
Lang-41-TBar-Patch\_2958\_1870 & 4 & T1:2, T3:2 & O:2, U:2 & \textcolor{orange}{O} \\
Lang-43-TBar-Patch\_368\_183 & 31 & T1:2, T3:2, NC:27 & O:10, U:21 & \textcolor{orange}{O} \\
Lang-44-TBar-Patch\_4046\_2567 & 10 & T3:1, NC:9 & O:2, U:8 & \textcolor{orange}{O} \\
Lang-45-TBar-Patch\_310\_221 & 15 & T1:2, T3:1, T4:3, NC:9 & O:7, U:8 & \textcolor{orange}{O} \\
Lang-51-TBar-Patch\_180\_129 & 54 & T3:50, T4:1, NC:3 & O:3, U:51 & \textcolor{orange}{O} \\
Lang-57-TBar-Patch\_44\_17 & 9 & T1:3, T2:2, T3:4 & C:5, U:4 & \textcolor{green!60!black}{C} \\
Lang-58-TBar-Patch\_1789\_1078 & 16 & T3:9, NC:7 & O:2, U:14 & \textcolor{orange}{O} \\
Lang-59-TBar-Patch\_1657\_1032 & 117 & T1:5, T3:112 & C:5, U:112 & \textcolor{green!60!black}{C} \\
Lang-60-TBar-Patch\_3262\_1865 & 6 & NC:6 & O:1, U:5 & \textcolor{orange}{O} \\
Lang-63-TBar-Patch\_28\_21 & 40 & NC:40 & U:40 & \textcolor{gray}{U} \\
Lang-7-TBar-Patch\_1504\_1083 & 64 & T1:2, T3:56, T4:3, NC:3 & C:5, U:59 & \textcolor{green!60!black}{C} \\
Math-11-TBar-Patch\_31\_8 & 1 & T3:1 & U:1 & \textcolor{gray}{U} \\
Math-15-TBar-Patch\_1163\_932 & 2 & T4:2 & O:2 & \textcolor{orange}{O} \\
Math-2-TBar-Patch\_468\_285 & 96 & T3:1, NC:95 & O:1, U:95 & \textcolor{orange}{O} \\
Math-5-TBar-Patch\_2\_2 & 30 & T1:11, T2:1, T3:17, NC:1 & C:12, U:18 & \textcolor{green!60!black}{C} \\
Math-50-TBar-Patch\_1\_1 & 103 & T3:100, T4:2, NC:1 & O:3, U:100 & \textcolor{orange}{O} \\
Math-57-TBar-Patch\_16\_7 & 15 & T1:9, T3:1, NC:5 & C:9, U:6 & \textcolor{green!60!black}{C} \\
Math-6-TBar-Patch\_5\_2 & 7 & T1:2, T2:4, T3:1 & O:6, U:1 & \textcolor{orange}{O} \\
Math-62-TBar-Patch\_261\_142 & 4 & T1:2, T4:1, NC:1 & O:3, U:1 & \textcolor{orange}{O} \\
Math-63-TBar-Patch\_611\_159 & 18 & T3:1, NC:17 & O:2, U:16 & \textcolor{orange}{O} \\
Math-65-TBar-Patch\_137\_80 & 1 & T3:1 & U:1 & \textcolor{gray}{U} \\
Math-70-TBar-Patch\_28\_28 & 70 & T1:22, T3:47, NC:1 & C:22, U:48 & \textcolor{green!60!black}{C} \\
Math-75-TBar-Patch\_3\_1 & 12 & T1:12 & C:12 & \textcolor{green!60!black}{C} \\
Math-79-TBar-Patch\_293\_124 & 6 & T1:5, T3:1 & C:5, U:1 & \textcolor{green!60!black}{C} \\
Math-8-TBar-Patch\_47\_16 & 113 & T3:1, T4:11, NC:101 & O:12, U:101 & \textcolor{orange}{O} \\
Math-80-TBar-Patch\_931\_596 & 98 & T1:2, T2:1, T3:15, NC:80 & O:3, U:95 & \textcolor{orange}{O} \\
Math-81-TBar-Patch\_75\_45 & 129 & T3:47, NC:82 & U:129 & \textcolor{gray}{U} \\
Math-82-TBar-Patch\_1326\_709 & 40 & T3:14, T4:10, NC:16 & O:19, U:21 & \textcolor{orange}{O} \\
Math-84-TBar-Patch\_114\_72 & 18 & T3:9, NC:9 & U:18 & \textcolor{gray}{U} \\
Math-85-TBar-Patch\_3\_1 & 60 & T1:7, T3:13, T4:4, NC:36 & O:19, U:41 & \textcolor{orange}{O} \\
Math-88-TBar-Patch\_593\_301 & 12 & T3:7, NC:5 & U:12 & \textcolor{gray}{U} \\
Math-89-TBar-Patch\_14\_12 & 7 & T1:2, T2:1, T3:4 & C:3, U:4 & \textcolor{green!60!black}{C} \\
Math-96-TBar-Patch\_439\_157 & 1 & NC:1 & O:1 & \textcolor{orange}{O} \\
Chart-2-TBar-patch1 & 68 & T1:15, T3:50, NC:3 & C:15, U:53 & \textcolor{green!60!black}{C} \\
Chart-11-TBar-patch1 & 12 & T1:7, T3:5 & C:7, U:5 & \textcolor{green!60!black}{C} \\
Chart-12-TBar-patch1 & 23 & T3:10, NC:13 & O:3, U:20 & \textcolor{orange}{O} \\
Chart-13-TBar-patch1 & 55 & T3:3, NC:52 & O:1, U:54 & \textcolor{orange}{O} \\
Chart-14-TBar-patch1 & 55 & T3:16, NC:39 & O:3, U:52 & \textcolor{orange}{O} \\
Chart-15-TBar-patch1 & 44 & T1:2, T3:31, NC:11 & O:2, U:42 & \textcolor{orange}{O} \\
Chart-24-TBar-patch1 & 12 & T1:6, T3:1, T4:5 & C:11, U:1 & \textcolor{green!60!black}{C} \\
Chart-25-TBar-patch1 & 99 & T1:2, T3:31, NC:66 & O:2, U:97 & \textcolor{orange}{O} \\
Chart-26-TBar-patch1 & 16 & T3:13, NC:3 & O:2, U:14 & \textcolor{orange}{O} \\
Chart-3-TBar-patch1 & 20 & T1:2, T3:8, NC:10 & O:3, U:17 & \textcolor{orange}{O} \\
Chart-5-TBar-patch1 & 23 & T3:19, NC:4 & U:23 & \textcolor{gray}{U} \\
Chart-7-TBar-patch1 & 20 & T1:3, T2:1, T3:4, NC:12 & O:6, U:14 & \textcolor{orange}{O} \\
Chart-8-TBar-patch1 & 10 & T1:3, T3:4, NC:3 & C:3, U:7 & \textcolor{green!60!black}{C} \\
Closure-107-TBar-patch1 & 2 & T3:2 & U:2 & \textcolor{gray}{U} \\
Closure-109-TBar-patch1 & 4 & T1:1, T3:1, NC:2 & O:1, U:3 & \textcolor{orange}{O} \\
Closure-115-TBar-patch1 & 37 & T3:36, NC:1 & U:37 & \textcolor{gray}{U} \\
Closure-12-TBar-patch1 & 7 & T1:2, NC:5 & O:3, U:4 & \textcolor{orange}{O} \\
Closure-126-TBar-patch1 & 44 & T3:44 & U:44 & \textcolor{gray}{U} \\
Closure-130-TBar-patch1 & 5 & NC:5 & O:1, U:4 & \textcolor{orange}{O} \\
Closure-21-TBar-patch1 & 53 & T3:53 & U:53 & \textcolor{gray}{U} \\
Closure-22-TBar-patch1 & 71 & T1:1, T3:70 & O:1, U:70 & \textcolor{orange}{O} \\
Closure-63-TBar-patch1 & 14 & T1:5, T3:9 & C:5, U:9 & \textcolor{green!60!black}{C} \\
Closure-66-TBar-patch1 & 4 & T1:2, NC:2 & O:3, U:1 & \textcolor{orange}{O} \\
Closure-73-TBar-patch1 & 10 & T1:8, T2:1, T3:1 & C:9, U:1 & \textcolor{green!60!black}{C} \\
Lang-11-TBar-patch1 & 8 & T1:2, T3:5, NC:1 & C:2, U:6 & \textcolor{green!60!black}{C} \\
Lang-12-TBar-patch1 & 4 & T1:2, NC:2 & O:2, U:2 & \textcolor{orange}{O} \\
Lang-18-TBar-patch1 & 3 & T1:2, T3:1 & O:2, U:1 & \textcolor{orange}{O} \\
Lang-19-TBar-patch1 & 6 & T3:6 & U:6 & \textcolor{gray}{U} \\
Lang-22-TBar-patch1 & 24 & T3:24 & U:24 & \textcolor{gray}{U} \\
Lang-23-TBar-patch1 & 8 & T1:2, NC:6 & O:8 & \textcolor{orange}{O} \\
Lang-25-TBar-patch1 & 18 & T1:2, T3:16 & O:2, U:16 & \textcolor{orange}{O} \\
Lang-34-TBar-patch1 & 8 & T3:7, T4:1 & C:1, U:7 & \textcolor{green!60!black}{C} \\
Lang-38-TBar-patch1 & 33 & T3:32, NC:1 & U:33 & \textcolor{gray}{U} \\
Lang-40-TBar-patch1 & 4 & T1:2, NC:2 & O:2, U:2 & \textcolor{orange}{O} \\
Lang-43-TBar-patch1 & 31 & T1:2, T3:11, NC:18 & O:10, U:21 & \textcolor{orange}{O} \\
Lang-44-TBar-patch1 & 10 & T3:9, NC:1 & O:1, U:9 & \textcolor{orange}{O} \\
Lang-47-TBar-patch1 & 15 & T1:2, T3:13 & O:2, U:13 & \textcolor{orange}{O} \\
Lang-53-TBar-patch1 & 54 & T3:54 & U:54 & \textcolor{gray}{U} \\
Lang-54-TBar-patch1 & 9 & T1:3, T3:6 & C:3, U:6 & \textcolor{green!60!black}{C} \\
Lang-55-TBar-patch1 & 16 & T3:16 & U:16 & \textcolor{gray}{U} \\
Lang-56-TBar-patch1 & 117 & T1:6, T3:111 & C:6, U:111 & \textcolor{green!60!black}{C} \\
Lang-61-TBar-patch1 & 6 & NC:6 & O:1, U:5 & \textcolor{orange}{O} \\
Lang-62-TBar-patch1 & 40 & T3:40 & U:40 & \textcolor{gray}{U} \\
Lang-8-TBar-patch1 & 64 & T1:2, T3:60, T4:2 & C:4, U:60 & \textcolor{green!60!black}{C} \\
Math-12-TBar-patch1 & 1 & T2:1 & C:1 & \textcolor{green!60!black}{C} \\
Math-14-TBar-patch1 & 2 & T3:2 & U:2 & \textcolor{gray}{U} \\
Math-1-TBar-patch1 & 96 & T3:1, NC:95 & O:1, U:95 & \textcolor{orange}{O} \\
Math-6-TBar-patch1 & 30 & T1:11, T2:2, T3:14, NC:3 & C:13, U:17 & \textcolor{green!60!black}{C} \\
Math-51-TBar-patch1 & 103 & T3:103 & U:103 & \textcolor{gray}{U} \\
Math-56-TBar-patch1 & 15 & T1:9, T3:1, NC:5 & C:9, U:6 & \textcolor{green!60!black}{C} \\
Math-6-TBar-patch1 & 7 & T1:2, T3:5 & O:2, U:5 & \textcolor{orange}{O} \\
Math-61-TBar-patch1 & 4 & T1:2, T3:2 & O:2, U:2 & \textcolor{orange}{O} \\
Math-64-TBar-patch1 & 18 & T3:3, NC:15 & O:2, U:16 & \textcolor{orange}{O} \\
Math-66-TBar-patch1 & 1 & T3:1 & U:1 & \textcolor{gray}{U} \\
Math-71-TBar-patch1 & 70 & T1:22, T3:48 & C:22, U:48 & \textcolor{green!60!black}{C} \\
Math-76-TBar-patch1 & 12 & T1:12 & C:12 & \textcolor{green!60!black}{C} \\
Math-78-TBar-patch1 & 6 & T1:5, T3:1 & C:5, U:1 & \textcolor{green!60!black}{C} \\
Math-8-TBar-patch1 & 112 & T3:112 & U:112 & \textcolor{gray}{U} \\
Math-80-TBar-patch1 & 98 & T1:2, T3:92, NC:4 & O:2, U:96 & \textcolor{orange}{O} \\
Math-81-TBar-patch1 & 129 & T3:129 & U:129 & \textcolor{gray}{U} \\
Math-82-TBar-patch1 & 40 & T3:40 & U:40 & \textcolor{gray}{U} \\
Math-84-TBar-patch1 & 18 & T1:1, T3:17 & O:1, U:17 & \textcolor{orange}{O} \\
Math-85-TBar-patch1 & 59 & T1:6, T3:53 & O:6, U:53 & \textcolor{orange}{O} \\
Math-88-TBar-patch1 & 12 & T3:7, NC:5 & U:12 & \textcolor{gray}{U} \\
Math-97-TBar-patch1 & 1 & T3:1 & U:1 & \textcolor{gray}{U} \\

\end{longtable}
